# Supplementary material for: Electron-phonon properties and superconductivity of doped antimonene
Source: arXiv:1806.08203 source file (2019-02-28)
Supplement: Supplementary file 1 [file supplement.pdf]

# SUPPLEMENTAL MATERIAL

## I. PHONON SPECTRUM WITH AND WITHOUT SOC CONSIDERATION

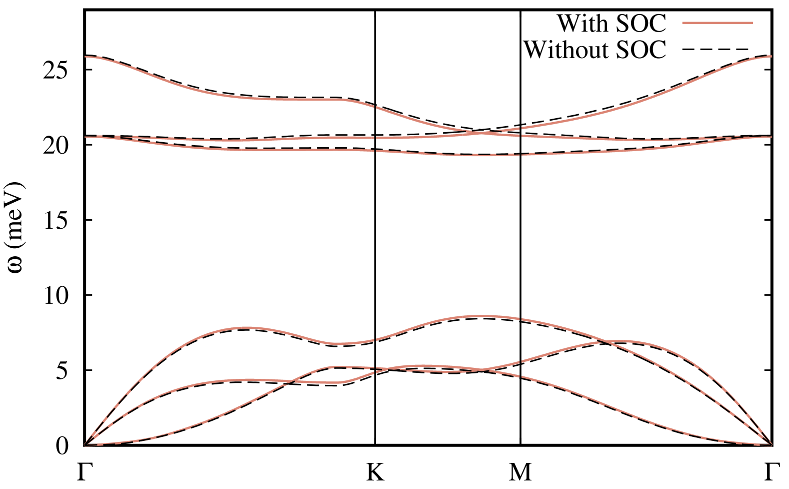


FIG. S1. Phonon spectrum of antimonene with SOC consideration (red line) and without (black dashed line).

## II. ELECTRON-PHONON COUPLING STRENGTH OF ELECTRON-DOPED ANTIMONENE

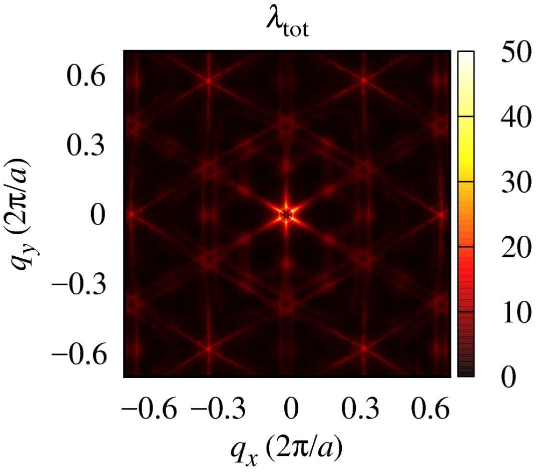


FIG. S2. Total electron-phonon coupling resolved in **q**-space at $N_e = 1 \times 10^{15}$ cm$^{-2}$.

## III. TABULATED DATA ON ELECTRON-PHONON COUPLING

Labels p correspond to the following modes in low **q** case: 2–$\lambda_{\mathrm{TA}}$, 3–$\lambda_{\mathrm{LA}}$, 4–TO, 5–LO, 6–$\lambda_{\mathrm{ZO}}$. $\lambda$ with index p = 1 is not presented, since the ZA mode was not considered in the electron-phonon coupling calculations. The $p$ indexes are ordered in order of increasing phonon energy.

TABLE S1. Single mode electron-phonon coupling strengths $\lambda_{\mathrm{p}}$ and average logarithmic phonon frequency for studied electron concentrations.

| $N_{\mathrm{e}}$ [cm$^{-2}$] | $\lambda_2$ | $\lambda_3$ | $\lambda_4$ | $\lambda_5$ | $\lambda_6$ | $\lambda$ | $\omega_{\log}$[K] |
|---|---|---|---|---|---|---|---|
| $5.0 \times 10^{12}$ | 0.042 | 0.072 | 0.114 | 0.087 | 0.037 | 0.352 | 106.5 |
| $1.0 \times 10^{13}$ | 0.063 | 0.078 | 0.120 | 0.091 | 0.040 | 0.392 | 100.1 |
| $5.0 \times 10^{13}$ | 0.077 | 0.078 | 0.127 | 0.093 | 0.045 | 0.419 | 114.3 |
| $1.0 \times 10^{14}$ | 0.359 | 0.268 | 0.118 | 0.088 | 0.050 | 0.883 | 83.1 |
| $2.0 \times 10^{14}$ | 0.396 | 0.341 | 0.156 | 0.092 | 0.073 | 1.058 | 87.5 |
| $4.0 \times 10^{14}$ | 0.707 | 0.423 | 0.226 | 0.135 | 0.100 | 1.592 | 85.7 |
| $5.0 \times 10^{14}$ | 0.511 | 0.374 | 0.183 | 0.122 | 0.092 | 1.281 | 90.2 |
| $7.0 \times 10^{14}$ | 0.465 | 0.317 | 0.158 | 0.154 | 0.111 | 1.205 | 94.6 |
| $1.0 \times 10^{15}$ | 0.670 | 0.646 | 0.293 | 0.347 | 0.387 | 2.342 | 104.8 |

TABLE S2. Single mode electron-phonon coupling strengths $\lambda_{\mathrm{p}}$ and average logarithmic phonon frequency for studied holes concentrations.

| $N_{\mathrm{e}}$ [cm$^{-2}$] | $\lambda_2$ | $\lambda_3$ | $\lambda_4$ | $\lambda_5$ | $\lambda_6$ | $\lambda$ | $\omega_{\log}$[K] |
|---|---|---|---|---|---|---|---|
| $5.0 \times 10^{12}$ | 0.006 | 0.022 | 0.002 | 0.002 | 0.033 | 0.066 | 67.0 |
| $1.0 \times 10^{13}$ | 0.006 | 0.032 | 0.006 | 0.007 | 0.033 | 0.085 | 96.2 |
| $5.0 \times 10^{13}$ | 0.061 | 0.076 | 0.044 | 0.061 | 0.043 | 0.285 | 103.9 |
| $1.0 \times 10^{14}$ | 0.051 | 0.074 | 0.033 | 0.059 | 0.035 | 0.251 | 88.5 |
| $2.0 \times 10^{14}$ | 0.123 | 0.333 | 0.020 | 0.049 | 0.050 | 0.576 | 85.9 |
| $2.5 \times 10^{14}$ | 0.363 | 0.880 | 0.019 | 0.044 | 0.150 | 1.457 | 81.5 |
| $3.0 \times 10^{14}$ | 0.931 | 1.839 | 0.021 | 0.047 | 0.342 | 3.180 | 79.4 |
| $3.7 \times 10^{14}$ | 1.788 | 2.693 | 0.023 | 0.045 | 0.493 | 5.041 | 79.0 |
| $4.0 \times 10^{14}$ | 1.528 | 1.847 | 0.022 | 0.036 | 0.352 | 3.785 | 81.3 |
| $5.0 \times 10^{14}$ | 0.685 | 0.806 | 0.022 | 0.034 | 0.183 | 1.731 | 87.7 |
| $1.0 \times 10^{15}$ | 0.394 | 0.451 | 0.074 | 0.049 | 0.163 | 1.131 | 89.6 |
